# Supplementary material for: Integrating Unimodal and Vision-Language Representations in Latent Space for Multi-Label Chest X-Ray Classification
Source: arXiv:2609.09185 source file (2026-08-31)
Supplement: Supplementary file 1 [file additional_results.tex]

\section{Additional experimental results}
\label{app:additional-results}

\subsection{Confirmatory statistical tests}
The complete paired-seed tests supporting the primary comparisons are reported
in Table 2 of the main paper. These values correspond to the
pre-specified confirmatory family described in the main paper.


\subsection{Expanded ablation interpretation}
The autoencoder and denoiser are interpreted as one latent-refinement block:
neither increment is significant alone, but their combination improves over
the embedding-only baseline. Holding that block fixed, pairwise differences
among the MLP, Transformer-only, gating-only, and Transformer-plus-gating
heads are nonsignificant. The latent-refinement gain is statistically
demonstrable only with Transformer plus gating, so the head is an enabling
condition rather than an independent gain source.

At the fusion stage, learned label-wise fusion of raw branches and a
capacity-matched CONCAT--MLP control both trail the full refined model. A deep
ensemble of three early-fusion models is statistically indistinguishable from
the full configuration, while outperforming a single early-fusion model.
Together with the leave-one-branch-out analysis, this indicates that the
method combines complementary representation sources, block-level latent
refinement, and an ensemble effect.

\subsection{Calibration analysis}
\label{app:calibration}
Because the fused outputs are normalized logits rather than probabilities,
we fit per-label Platt scaling on the validation set and evaluate expected
calibration error (ECE) and Brier score on the test set. All configurations
are well calibrated after scaling, with ECE $\leq 0.014$. Fusion improves the
Brier score relative to the RAD-DINO and BioViL-T single-source models
($0.0832$ versus $0.0858$ and $0.0887$), although its ECE ($0.0140$) is
slightly higher than their $0.0125$ values.

\input{tables/06_calibration}

\subsection{Performance by label prevalence}
\label{app:prevalence}
We stratify the 14 labels into common ($>15\%$, 8 labels), mid-prevalence
($5$--$15\%$, 3 labels), and rare ($<5\%$, 3 labels) tiers, then compare
hybrid and early fusion with per-label bootstrap intervals. The improvement
is well supported on common labels for both metrics and is less uniform in
the middle tier. For rare labels, AUROC intervals exclude zero for all three,
whereas no AP interval does, reflecting the small number of positive studies.
The rare labels also have the lowest between-branch error correlations,
leaving more residual disagreement for fusion to exploit.

\input{tables/07_prevalence}
